# Supplementary material for: Tunability of domain structure and magnonic spectra in antidot arrays of Heusler alloy
Source: arXiv:1907.02746 source file (2019-07-05)
Supplement: Supplementary file 1 [file Bedanta_Supplementary_Information_PRA_rev.pdf]

# Supplemental Material:
# Tunability of domain structure and magnonic spectra in antidot arrays of Heusler alloy


Sougata Mallick,[1] Sucheta Mondal,[2] Takeshi Seki,[3,4] Sourav Sahoo,[2] Thomas Forrest,[5] Francesco Maccherozzi,[5] Zhenchao Wen,[3,4,*] Saswati Barman,[6] Anjan Barman,[2] Koki Takanashi,[3,4] and Subhankar Bedanta[1,†]

[1] *Laboratory for Nanomagnetism and Magnetic Materials (LNMM), School of Physical Sciences, National Institute of Science Education and Research, HBNI, Jatni-752050, Odisha, India*

[2] *Department of Condensed Matter Physics and Material Sciences, S. N. Bose National Centre for Basic Sciences, Block JD, Sector III, Salt Lake, Kolkata 700106, India*

[3] *Institute for Materials Research, Tohoku University, Sendai 980-8577, Japan*

[4] *Center for Spintronics Research Network, Tohoku University, Sendai 980-8577, Japan*

[5] *Diamond Light Source Ltd., Diamond House, Didcot, Oxfordshire, OX11 0DE, UK*

[6] *Institute of Engineering and Management, Sector V, Salt Lake, Kolkata 700091, India*


TABLE ST1. Detail description of the samples

| Name | Type | Feature size |
|---|---|---|
| Sample TF | Thin film | - |
| Sample CA | Circular antidot | Diameter : 200 nm |
| Sample SA | Square antidot | Side length : 200 nm |
| Sample TA | Triangular antidot | Side length : 200 nm |
| Sample SA | Diamond antidot | Side length : 200 nm |

## Microfabrication of the MAL arrays:

Patterning on the thin film was performed using e-beam lithography followed by development in isopropanol and distilled water for 7 and 20 seconds, successively. Ar ion milling was performed at $6 \times 10^{-7}$ mbar to etch out the residual films. Finally, the MAL arrays were obtained by developing the films in pyrrolidone for 4 hours. The feature size of the holes and the center to center distance between the holes are 200 and 400 nm, respectively. The detailed list of all the samples discussed in this paper is presented in table ST1. Figure S1 shows the orientation of the easy axis and applied field with the crystallographic axes of MgO substrate and CFMS thin film in the antidot array.

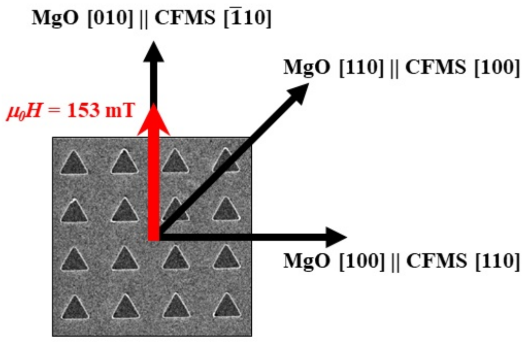


FIG. S1. Schematic showing the orientation of easy axes, and applied field with the crystallographic axes of MgO substrate and CFMS film in the antidot array.

## Anisotropy behavior of the continuous thin film (TF):

Figure S2(a) shows the angular dependence of coercive field plot for TF. The values of $H_C$ have been extracted from the angle dependent hysteresis measurements performed using micro-MOKE. Here the magnetic field was applied at various angles ($\phi$) to the easy axis, i.e. along CFMS [$\bar{1}$10]. The easy axes (maximum $H_C$) at 0°, 90°, 180°, and 270° reveal that the film exhibits anisotropy with cubic symmetry. However, it should be noted that the position of all the hard axes are not well defined. There are two minima at 135°, and 315° which are the ideal positions for the hard axes with cubic symmetry. Nevertheless, minima along 60° and 240° are shifted from the original hard axes position of 45°, and 225°. Further, the strengths of $H_C$ along all the easy axes are unequal. This indicates presence of another type of anisotropy (uniaxial), superimposed on the cubic one. The uniaxial anisotropy has its easy axes along 0°, and 180°, separated by the hard axes along 90°, and 270°. This leads to shift of the minima in the coercivity plot to 60°, and 240°, respectively.

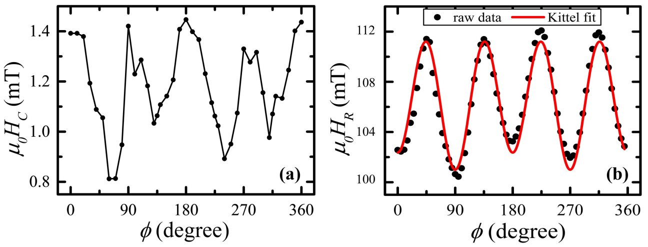


FIG. S2. (a) Angular ($\phi$) dependence of coercivity plot for TF measured using micro-MOKE in longitudinal mode. (b) Angular dependence of resonance field ($H_R$) plot for TF extracted from the FMR measurements. The black dots represent the experimental data points whereas the red line represents the best fit curve using Kittel equation with two anisotropy model.


* Present address: National Institute for Materials Science, Tsukuba 305-0047, Japan

† sbedanta@niser.ac.in

In order to quantify the strength of the uniaxial and cubic anisotropies, we have performed angle dependent FMR measurements on TF at the frequency of 10 GHz. We have plotted the resonance field ($H_R$) as a function of the angle ($\phi$) to obtain the anisotropy behavior. Figure S2(b) shows the angular dependent resonance field data fitted with eqn. 1 for TF. The strength of uniaxial and cubic anisotropies have been extracted by fitting the angular dependent FMR data with two anisotropy Kittel equation. The fitted values of $K_2$ and $K_4$ are $0.34 \times 10^3$, and $1.2 \times 10^3 J/m^3$, respectively. Hence, it can be concluded that a noticeable contribution of uniaxial anisotropy is present in TF, which is $\sim$ 28% of the dominant cubic anisotropy. The uniaxial anisotropy can be introduced in a film due to several reasons viz. oblique angular deposition, anisotropic strain relaxation, miscut in the substrate, interfacial roughness, interfacial alloy formation, growth on a stepped substrate, etc. [1–4] The presence of such strong uniaxial anisotropy leads to the shift in the position of the hard axes as observed in figure S2(a). We have further extracted the damping constant ($\alpha$) = 0.0056 from the frequency dependent FMR measurements. The parameters extracted from the FMR measurements have been used in OOMMF simulation.

## Precessional dynamics measurement using TR-MOKE:

The ultrafast magnetization dynamics of the samples was measured using an all optical TR-MOKE microscope set-up in pump-probe geometry.[5, 6] We have used the second harmonic ($\lambda$ = 400 nm, fluence = 10 $mJ/cm^2$, pulse width $\sim$100 fs) to pump the samples. A time delayed fundamental laser beam ($\lambda$ = 800 nm, avg. power= 2.5 mW) (Model: Tsunami from Spectraphysics) has been used to probe the precessional signal by measuring the polar Kerr rotation. The probe beam has a spot size of 800 nm whereas the pump beam is spatially superimposed with the probe. Magnetic fields with the amplitude significantly higher than the saturation fields of the samples have been applied in-plane to ensure the magnetization pointing towards the bias field orientation. A mechanical chopper working at 2 kHz frequency has been used to chop the pump beam for phase sensitive detection of the Kerr rotation signal.
The experimental precessional data (background subtracted) of the time-resoled magneto-optical Kerr rotation for TF at $\mu_0 H$ = 153 mT, is shown in figure S3(a). Figure S3(b) shows the corresponding FFT power spectrum which yields a precessional frequency of 12.51 GHz at $\mu_0 H$ =153 mT. Figure S3 (c) - (d) show the Kerr rotation and corresponding FFT spectrum for the aforementioned field obtained by OOMMF simulation. From figure S3 (b), and (d), it can be concluded that the simulated precessional frequency matches (within the error bar) with the experimental observation. Figure S3 (e) shows the experimental and simulated precessional frequency plot as a function of amplitude of applied magnetic field. This further confirms that the experimental and simulated frequency matches well within the experimental field range. The experiment as well as the simulations for the antidot samples have been performed at $\mu_0 H$ =153 mT.

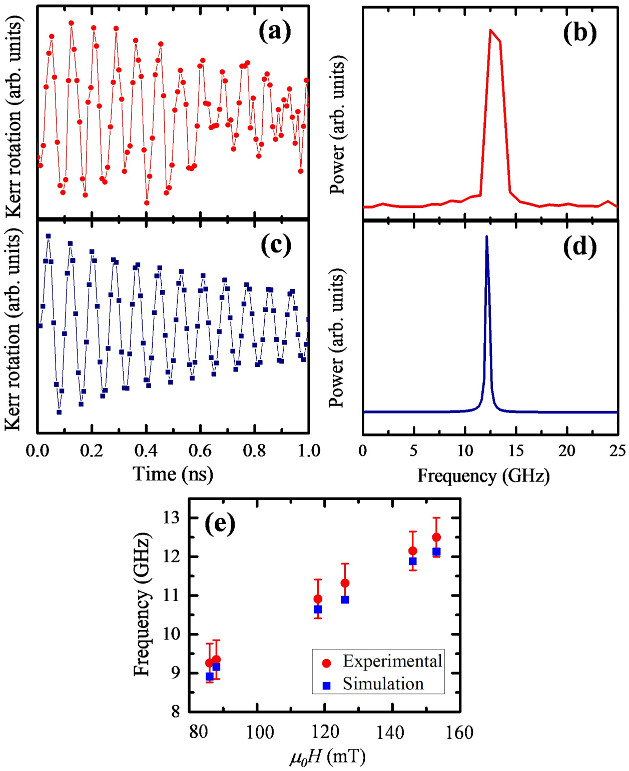


FIG. S3. Experimentally observed time resolved Kerr rotation data (a) and corresponding FFT spectra (b) for the continuous thin film (TF) at $\mu_0 H$ = 153 mT. Similarly, (c) and (d) shows the OOMMF simulated Kerr rotation and the corresponding FFT spectra, respectively, at the same applied field. Figure (e) shows the extracted precessional frequency as a function of the external field for both experiment (red dots) and simulation (blue squares).

## Simulated phase maps of the antidot arrays (CA, SA, TA, and DA):

Figure S4 shows the simulated phase maps for the precessional modes for circular, square, triangular, and diamond antidots (CA, SA, TA, and DA).

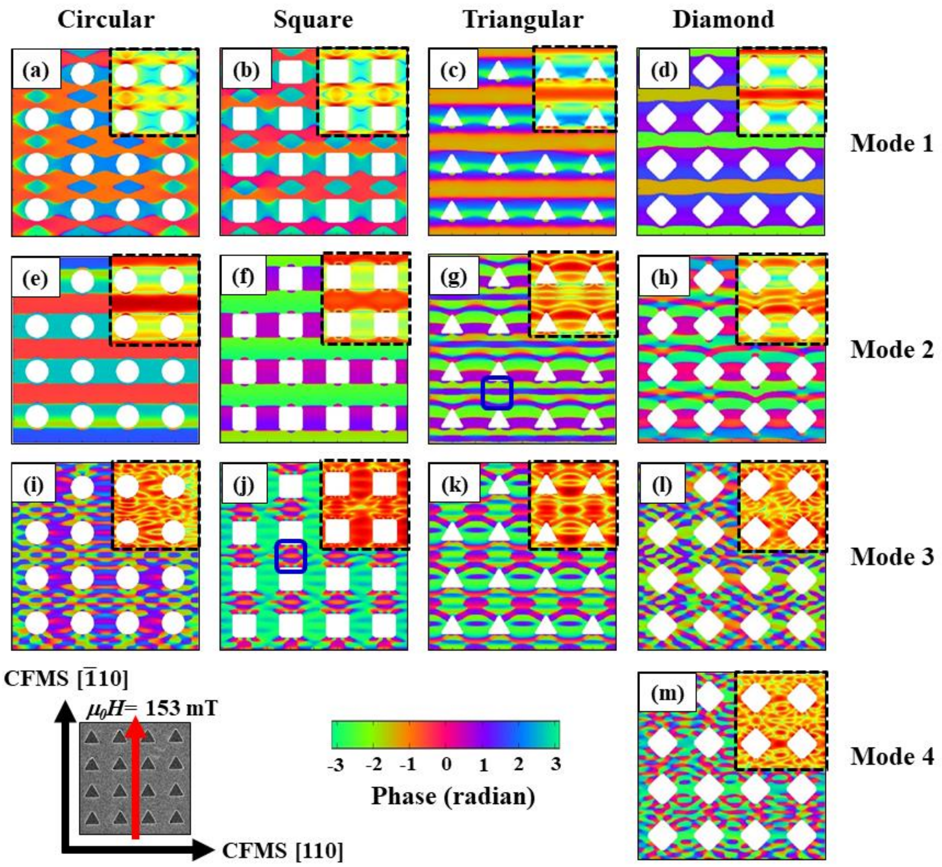


FIG. S4. Simulated phase maps for different precessional modes as shown in figure 4 (e) - (h) for CA, SA, TA, and DA, respectively. The color map for the phase distribution is shown at the right top of the image. The respective mode numbers as per figure 4 is shown at the bottom of the image. An external magnetic field of 153 mT is applied along the easy axis (CFMS [$\bar{1}$10]).


[1] Y. B. Xu, D. J. Freeland, M. Tselepi, and J. A. C. Bland, Anisotropic lattice relaxation and uniaxial magnetic anisotropy inFe/InAs(100)42, Phys. Rev. B **62**, 1167 (2000).

[2] Q. F. Zhan, S. Vandezande, C. Van Haesendonck, and K. Temst, Manipulation of in-plane uniaxial anisotropy in Fe/MgO(001) films by ion sputtering, Appl. Phys. Lett. **91**, 122510 (2007).

[3] O. Thomas, Q. Shen, P. Schieffer, N. Tournerie, and B. Lepine, Interplay between anisotropic strain relaxation and uniaxial interface magnetic anisotropy in epitaxial Fe films on (001) GaAs, Phys. Rev. Lett. **90**, 017205 (2003).

[4] S. Mallick, S. Mallik, B. B. Singh, N. Chowdhury, R. Gieniusz, A. Maziewski, and S. Bedanta, Tuning the anisotropy and domain structure of Co films by variable growth conditions and seed layers, J. Phys. D: Appl. Phys. **51**, 275003 (2018).

[5] R. Mandal, P. Laha, K. Das, S. Saha, S. Barman, A. K. Raychaudhuri, A. Barman, Effects of antidot shape on the spin wave spectra of two-dimensional Ni80Fe20 antidot lattices, Appl. Phys. Lett. **103**, 262410 (2013).

[6] R. Mandal, S. Saha, D. Kumar, S. Barman, S. Pal, K. Das, A. K. Raychaudhuri, Y. Fukuma, Y. Otani, and A. Barman, Optically induced tunable magnetization dynamics in nanoscale co antidot lattices, ACS Nano **6**, 3397 (2012).
